# Supplementary material for: Syntactic Language Change in English and German: Metrics, Parsers, and Convergences
Source: arXiv:2402.11549 source file (2024-03-28)
Supplement: Supplementary file 1 [file 999_appendix.tex]

\section{Appendix}
%\iffalse
%\clearpage
%\subsection{Annotation Guidelines}\label{app:anno}
%\clearpage
%\includepdf[pages=1-2,scale=.75,picturecommand*={\put (\LenToUnit{.05\paperwidth},20) {};}]{figs/annotation_guidelines.pdf}

\begin{figure*}[h]
	\centering
 \hspace*{-2cm}
 \vspace*{-2cm}
  \includegraphics[page=2,height=1.3\textwidth,angle=90]
 {figs/annotation_guidelines.pdf}
 \hspace*{-2cm}
	\includegraphics[page=1,height=1.3\textwidth,angle=90]{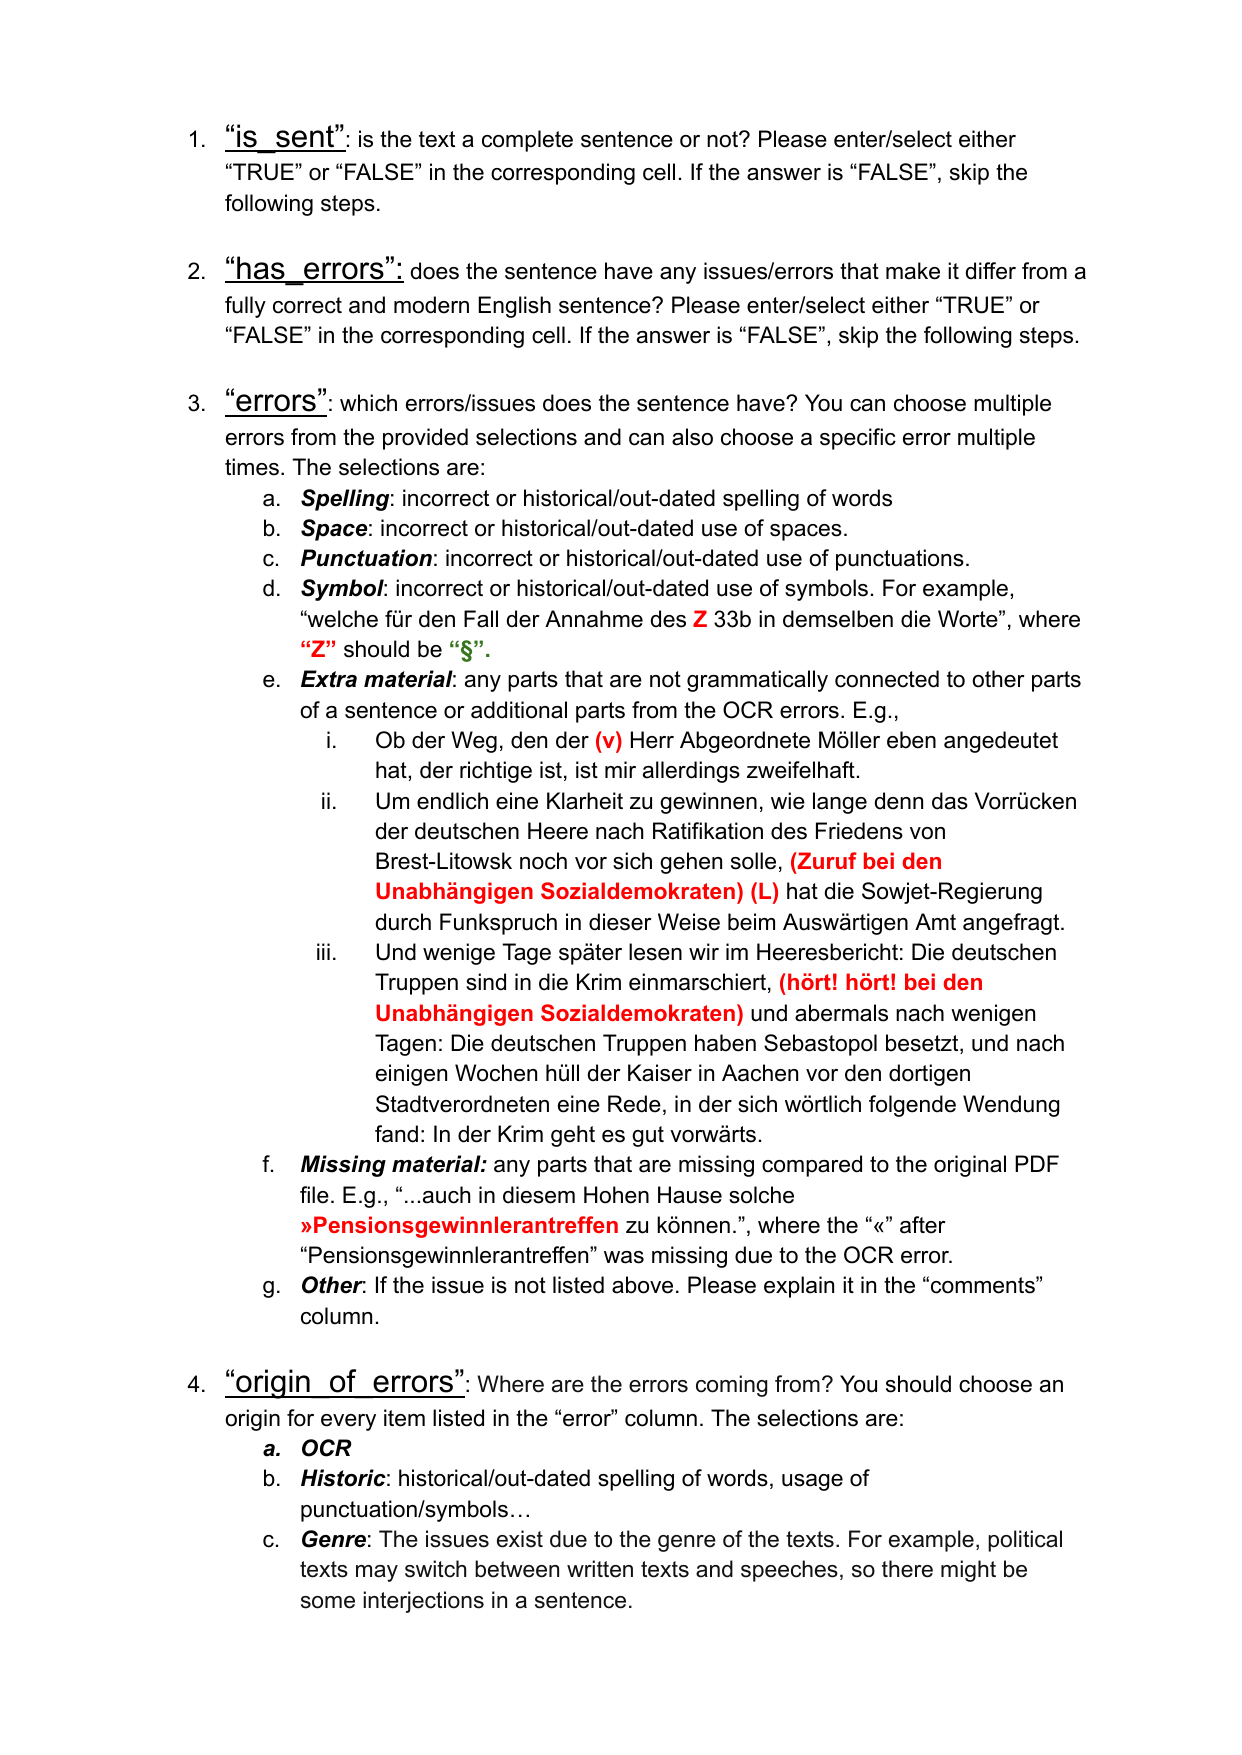}
	\caption{Annotation Guidelines for Hansard.}
	\label{fig:guideline}
\end{figure*}

\iffalse
\begin{landscape} % Be sure to wrap in 'landscape' environment
\includepdf[
    pages=-,                
    nup=1x2,                
    frame,                  
    landscape,          
    delta=5mm 5mm,  
    scale=0.90,
    % Set the caption on the first page of output
    pagecommand*={\thispagestyle{plain}\null\vfill\captionof{figure}{This is the SECOND caption}},
    % Set the [continued] caption on second and subsequent pages
    % Use '\captionof*{...} to avoid duplicate entries in listoffigures
    pagecommand={\thispagestyle{plain}\null\vfill\captionof*{figure}{\figurename~\thefigure: This is the SECOND caption (Continued)}}
]{figs/annotation_guidelines.pdf}
\end{landscape}
\fi
